# Supplementary material for: Semantic Shield: Defending Vision-Language Models Against Backdooring and Poisoning via Fine-grained Knowledge Alignment
Source: arXiv:2411.15673 source file (2024-11-23)
Supplement: Supplementary file 3 [file qual_img.tex]

\section{Qualitative Analysis}
\label{supple_sec:qual}
In \cref{fig:qual_analysis_supple}, we present illustrative examples of attention maps for both backdoored models and our defended model (weighted CL + attention). In \cref{fig:patch_image1} and \cref{fig:patch_image2}, a small backdoor trigger is introduced to the bottom right corner of the image. It is evident that the backdoored models focus their attention on the backdoor trigger in \cref{fig:patch_map1} and \cref{fig:patch_map2} (highlighting the bottom right part of the image). Conversely, our defended model (weighted CL + attention) exhibits no attention in the bottom right part of the images, as observed in \cref{fig:patch_model1} and \cref{fig:patch_model2}.

Next, we conducted experiments on our model's performance with two types of visually imperceptible examples, namely BPP \cite{bpp} and WANet \cite{wanet} (refer to \cref{fig:bpp_image1}, \cref{fig:bpp_image2}, \cref{fig:wanet_image1}, \cref{fig:wanet_image2}). We introduced noise throughout the images to deceive traditional visual language models, as these models tend to pay attention all over the images (\cref{fig:bpp_map1}, \cref{fig:bpp_map2} for BPP, \cref{fig:wanet_map1}, \cref{fig:wanet_map2} for Wanet). In contrast, our models focus their attention on the expected regions, ignoring all noisy areas of the images (\cref{fig:bpp_model1}, \cref{fig:bpp_model2} for BPP, \cref{fig:wanet_model1}, \cref{fig:wanet_model2} for Wanet).
