# Supplementary material for: Semantic Shield: Defending Vision-Language Models Against Backdooring and Poisoning via Fine-grained Knowledge Alignment
Source: arXiv:2411.15673 source file (2024-11-23)
Supplement: Supplementary file 5 [file introduction.tex]

\section{Introduction}
\label{supple_sec:intro}

We offer supplementary results complementing those presented in our main paper. Initially, we describe the process of generating knowledge elements from Vicuna \cite{vicuna} in \cref{supple_sec:prompt_gen}. Subsequently, we conduct a comparison between our model and a new model, RoCLIP \cite{roclip}, as outlined in \cref{supple_sec: experiments}. Finally, we provide additional qualitative analysis comparing the poisoned model to our model, demonstrating attention maps in \cref{supple_sec:qual}.
