# Supplementary material for: Semantic Shield: Defending Vision-Language Models Against Backdooring and Poisoning via Fine-grained Knowledge Alignment
Source: arXiv:2411.15673 source file (2024-11-23)
Supplement: Supplementary file 6 [file experiments_rebuttal.tex]

% Reviewer WYZL
% The study proposes four loss functions: CL, KE, Attention, and Weighted CL, which can lead to numerous combinations of losses. However, the experiment section only presents the results for CL + KE, CL + Attention, and Weighted CL + Attention. It would be beneficial to explore other potential combinations, such as Weighted CL + KE and Weighted CL + Attention + KE, to provide a more comprehensive understanding of their impact on the defense's performance.

## weighted CL + KE
## weighted CL + attention + KE

 % In the experiment section, the results for CL + KE, CL + Attention, and Weighted CL + Attention are presented. These loss functions require the assignment of different weights. It would be beneficial to delve into the sensitivity of these parameters.

 ## lambda1 and lambda2 

 acc vs \lambda 1 vs \lambda 2. The graph should be \lambda 2 vs hit@10 (attack), and \lambda 2 vs clean acc

 
